# Supplementary material for: GraphTango: A Hybrid Representation Format for Efficient Streaming Graph Updates and Analysis
Source: arXiv:2212.11935 source file (2022-12-22)
Supplement: Supplementary file 1 [file appendix.tex]

\appendix

\section{Hash Function Implementation}
\label{app:hash}

Given these parameters,

    $M=$ Number of cache lines in the hash table
    
    $N=$ Number of $\{key,value\}$ pairs within a cache line

Our proposed hash function is of the following form:
\begin{equation*}
    h(key,i)=N \cdot h_1\left(key, \left\lfloor \frac{i}{N} \right\rfloor\right) + h_2(key, i~mod~N)
\end{equation*}

Here, $h_1()$ selects a cache line inside the hash table array, and $h_2()$ selects an offset within the cache line. Therefore, $h_1()$ must be a permutation of $\{0,1,...,M-1\}$ to ensure that all cache lines are eventually selected. Similarly, $h_2()$ must be a permutation of $\{0,1,...,N-1\}$ to explore all $\{key,value\}$ pairs within a cache line. Any $h_1()$ and $h_2()$ that meet the permutation requirement can be used. For \gname{}, we used the following:
\begin{align*}
    h_1(k, x)   &=  (h_3(k) + x \cdot h_4(k))~mod~M   \\
    h_2(k, x)   &= (k+x)~mod~N          \\
    h_3(k)      &= \lfloor(A \cdot k~mod~2^w)/2^{w-m}\rfloor    \\
    h_4(k)      &= \lfloor(A \cdot k~mod~2^w)/2^{w-2m}\rfloor ~or~1    
\end{align*}

Here, 
% \begin{align*}
%     A &= A~multiplicative~constant \\
%     w &= key~width~in~bits \\
%     m &= log_2(M)
% \end{align*}
$w$ is the key width in bits, $A$ is a large constant, and $m = log_2(M)$. We use double hashing for $h_1()$ to negate primary/secondary clustering. It is computed with the help of two pairwise independent hashing functions, $h_3()$ and $h_4()$. $h_3()$ and $h_4()$ are computed with multiplicative hashing. As for $h_2()$, we used simple linear probing. Although seemingly complex, the hash can be computed cheaply as we ensure both $N$ and $M$ are powers of two. The following code snippet shows how to calculate the hash value for a 32-bit key:
%\begin{lstlisting}[language=C]
\begin{minted}
[
frame=lines,
framesep=1mm,
%baselinestretch=1.1,
bgcolor=LightGray,
fontsize=\footnotesize,
]
{C}
u32 h(u32 key, u32 i){
    u32 y = key * A;
    u32 h3 = y >> (32 - logM);
    u32 h4 = (y >> (32 - (logM << 1))) | 1;
    u32 h1 = (h3 + (i >> logN) * h4) & (M - 1);
    u32 h2 = (key + i) & (N - 1);
    return (h1 << logN) + h2;
}
\end{minted}
%\end{lstlisting}

Note that the code does not need any expensive division/modulus operation. When compiled on an x86\_64 machine with gcc 9.3.0 and -O3 flag, it resulted in 2 multiplications and 8 other simple arithmetic/logical instructions.
